# Supplementary material for: Using high multipolar orders to reconstruct the sound velocity in piezoelectrics from lattice dynamics
Source: arXiv:2004.08875 ancillary file (2020-04-19)
Supplement: Supplementary file 1 [file Supplemental.pdf]

# Supplemental Material for "Using high multipolar orders to reconstruct the sound velocity in piezoelectrics from lattice dynamics"


Miquel Royo,[1] Konstanze R. Hahn,[1] and Massimiliano Stengel[1,2]

[1] *Institut de Ciència de Materials de Barcelona (ICMAB-CSIC), Campus UAB, 08193 Bellaterra, Spain*
[2] *ICREA - Institució Catalana de Recerca i Estudis Avançats, 08010 Barcelona, Spain*


(Dated: April 19, 2020)

**Multipolar electrostatic interactions.** We shall recap the discussion of the macroscopic electrostatic contributions to the long-wavelength dynamical matrix, by mostly following the discussion of Ref. [1]. First, we decompose the dynamical matrix into its analytic (AN) and nonanalytic (NA) contributions,

$$\Phi(\mathbf{q}) = \Phi^{\rm AN}(\mathbf{q}) + \Phi^{\rm NA}(\mathbf{q}), \tag{S.1}$$

where the NA part carries the macroscopic electric field effects. The latter manifest themselves as long-ranged interatomic forces in real space, and can be expressed as [2]

$$\Phi^{\rm NA}(\mathbf{q}) = \frac{4\pi}{\Omega}\frac{|\mathcal{Q}(\mathbf{q})\rangle\langle\mathcal{Q}(\mathbf{q})|}{\xi(\mathbf{q})}. \tag{S.2}$$

Note that the charge response to a phonon, $|\mathcal{Q}(\mathbf{q})\rangle$, and the dielectric screening function, $\xi(\mathbf{q})$, are both analytic functions of $\mathbf{q}$. [The nonanaliticity of $\Phi^{\rm NA}(\mathbf{q})$ arises from the fact that $\xi(\mathbf{q})$ vanishes quadratically in a vicinity of $\Gamma$.] Thus, in the long-wavelength limit they can be expanded as [1]

$$\begin{aligned}\mathcal{Q}_{\kappa\beta}(\mathbf{q}) =& -iq_\gamma Q^{(1,\gamma)}_{\kappa\beta} - \frac{q_\gamma q_\delta}{2} Q^{(2,\gamma\delta)}_{\kappa\beta} \\ &+ i\frac{q_\gamma q_\delta q_\sigma}{3!} Q^{(3,\gamma\delta\sigma)}_{\kappa\beta} + \dots,\end{aligned} \tag{S.3}$$

and

$$\xi(\mathbf{q}) = \mathbf{q}\cdot\boldsymbol{\epsilon}^{(2)}\cdot\mathbf{q} + \mathbf{q}\mathbf{q}\cdot\boldsymbol{\epsilon}^{(4)}\cdot\mathbf{q}\mathbf{q} + \dots \tag{S.4}$$

Here $Q^{(n,\dots)}_{\kappa\beta}$, are the Cartesian components of the dynamical multipole tensors of order $n$ associated to the displacement of an atom $\kappa$ along $\beta$, respectively dynamical dipoles (also known as Born effective charges, $n = 1$), quadrupoles [3] ($n = 2$) and octupoles ($n = 3$). $\boldsymbol{\epsilon}^{(2)}$ stands for the electronic (clamped-ion) dielectric tensor, while $\boldsymbol{\epsilon}^{(4)}$ describes the spatial dispersion of the latter.

We are ready now to perform a multipolar expansion of $\Phi^{\rm NA}(\mathbf{q})$, for which we shall introduce the following shorthand notation,

$$\langle\kappa\beta|Z(\mathbf{q})\rangle = \sum_\gamma q_\gamma Q^{(1,\gamma)}_{\kappa\beta}, \tag{S.5}$$

$$\langle\kappa\beta|Q(\mathbf{q})\rangle = \sum_{\gamma\delta} q_\gamma q_\delta Q^{(2,\gamma\delta)}_{\kappa\beta}, \tag{S.6}$$

$$\langle\kappa\beta|O(\mathbf{q})\rangle = \sum_{\gamma\delta\lambda} q_\gamma q_\delta q_\lambda Q^{(3,\gamma\delta\lambda)}_{\kappa\beta}. \tag{S.7}$$

By using the above expansions of the charge and dielectric response we find, at the lowest orders in $q$,

$$\Phi^{\rm DD}(\mathbf{q}) = \frac{4\pi}{\Omega}\frac{|Z(\mathbf{q})\rangle\langle Z(\mathbf{q})|}{\mathbf{q}\cdot\boldsymbol{\epsilon}\cdot\mathbf{q}}, \tag{S.8}$$

$$\Phi^{\rm DQ}(\mathbf{q}) = -i\frac{4\pi}{2\Omega}\frac{|Z(\mathbf{q})\rangle\langle Q(\mathbf{q})| + |Q(\mathbf{q})\rangle\langle Z(\mathbf{q})|}{\mathbf{q}\cdot\boldsymbol{\epsilon}\cdot\mathbf{q}}, \tag{S.9}$$

$$\Phi^{\rm DO}(\mathbf{q}) = -\frac{4\pi}{6\Omega}\frac{|Z(\mathbf{q})\rangle\langle O(\mathbf{q})| + |O(\mathbf{q})\rangle\langle Z(\mathbf{q})|}{\mathbf{q}\cdot\boldsymbol{\epsilon}\cdot\mathbf{q}}, \tag{S.10}$$

$$\Phi^{\rm QQ}(\mathbf{q}) = \frac{4\pi}{4\Omega}\frac{|Q(\mathbf{q})\rangle\langle Q(\mathbf{q})|}{\mathbf{q}\cdot\boldsymbol{\epsilon}\cdot\mathbf{q}}, \tag{S.11}$$

$$\Phi^{\rm D\epsilon D}(\mathbf{q}) = -\frac{4\pi}{\Omega}\frac{|Z(\mathbf{q})\rangle\,(\mathbf{q}\,\mathbf{q}\cdot\boldsymbol{\epsilon}^{(4)}\cdot\mathbf{q}\,\mathbf{q})\,\langle Z(\mathbf{q})|}{(\mathbf{q}\cdot\boldsymbol{\epsilon}\cdot\mathbf{q})^2}, \tag{S.12}$$

The above expansion terms only concern the macroscopic part of the multipolar interactions. For practical use in the Fourier interpolation procedure, we recast them as interactions between Gaussian multipoles, following standard Ewald techniques. [4] In particular, we perform a summation over the reciprocal-space Bravais lattice of $\mathbf{G}$ vectors of the form

$$\hat{C}^{\rm LR}_{\kappa\alpha,\kappa'\beta}(\mathbf{q}) = \sum_{\mathbf{G}}{}' \langle\kappa\alpha|\Phi^{\rm mac}(\mathbf{q}+\mathbf{G})|\kappa'\beta\rangle\, e^{-i\mathbf{G}\cdot(\boldsymbol{\tau}_{\kappa'}-\boldsymbol{\tau}_{\kappa})}\, e^{-\frac{|\mathbf{G}+\mathbf{q}|^2}{\Lambda^2}}, \tag{S.13}$$

where the primed sum indicates that terms with $\mathbf{G}+\mathbf{q}=0$ are excluded, and

$$\Phi^{\rm mac}(\mathbf{q}) = \Phi^{\rm DD}(\mathbf{q}) + \Phi^{\rm DQ}(\mathbf{q}) + \Phi^{\rm DO}(\mathbf{q}) + \Phi^{\rm QQ}(\mathbf{q}) + \Phi^{\rm D\epsilon D}(\mathbf{q}). \tag{S.14}$$

In principle, a strict application of the Ewald method would imply a real-space sum to be included as well, with $\Lambda$ set to an optimal value that minimizes the computational burden. In our implementation we decided to avoid the real-space part altogether, since we found it to be irrelevant provided that a sufficiently large value of $\Lambda$ is used. (The width of the Gaussian multipoles should be an order of magnitude smaller than the size of the supercell that is used to represent the IFC.) In particular, for the calculations reported in the manuscript we have used a value of 1 Bohr$^{-1}$ for $\Lambda$ which, for the studied $BaTiO_3$ system, corresponds to a real-space Gaussian width of 2.46 Bohr.

In addition, a smooth fulfillment of the acoustic sum rule was enforced as follows, [4]

$$\Phi^{\rm LR}_{\kappa\alpha,\kappa'\beta}(\mathbf{q}) = \hat{C}^{\rm LR}_{\kappa\alpha,\kappa'\beta}(\mathbf{q}) - \delta_{\kappa\kappa'}\sum_{\kappa''}\hat{C}^{\rm LR}_{\kappa\alpha,\kappa''\beta}(\mathbf{q}=0), \tag{S.15}$$

with $\Phi^{\rm LR}_{\kappa\alpha,\kappa'\beta}(\mathbf{q})$ being the final long-range dynamical matrix used in Eq. (10) of the manuscript.

**Derivation of the Christoffel equation from the microscopic force constants.** Here we shall provide a formal proof that Eq.(4) of the main text indeed leads to the eigenvalue problem for the macroscopic sound velocity written in terms of the generalized elastic tensor, i.e., we will prove the validity of Eq.(7). We shall first of all introduce the following definitions,

$$\Lambda^{\kappa}_{\alpha\beta}(\hat{\mathbf{q}}) = \sum_{\kappa'}\phi^{(1,\hat{\mathbf{q}})}_{\kappa\alpha,\kappa'\beta}, \tag{S.16}$$

$$\bar{K}^{\hat{\mathbf{q}}}_{\alpha\beta} = -\frac{1}{2}\sum_{\kappa\kappa'}\phi^{(2,\hat{\mathbf{q}})}_{\kappa\alpha,\kappa'\beta}. \tag{S.17}$$

This way, Eqs. (5) and (6) of the main text can be rewritten as

$$K^{\hat{\mathbf{q}}}_{jl} = \bar{K}^{\hat{\mathbf{q}}}_{jl} - \sum_{\kappa\kappa'\alpha\beta}\Lambda^{\kappa}_{\alpha j}(\hat{\mathbf{q}})\,\widetilde{\Phi}^{(0,\hat{\mathbf{q}})}_{\kappa\alpha,\kappa'\beta}\,\Lambda^{\kappa'}_{\beta l}(\hat{\mathbf{q}}). \tag{S.18}$$

Now we can proceed to decomposing $K^{\hat{\mathbf{q}}}_{jl}$ into an analytic and nonanalytic part based on the analogous decomposition of the dynamical matrix discussed in the previous Section. The first term is relatively easy to work out,

$$\bar{K}^{\hat{\mathbf{q}}}_{jl} = \bar{K}^{\rm AN,\hat{\mathbf{q}}}_{jl} + \frac{4\pi}{4\Omega}\frac{Q^{\hat{\mathbf{q}}}_j Q^{\hat{\mathbf{q}}}_l}{\hat{\mathbf{q}}\cdot\boldsymbol{\epsilon}\cdot\hat{\mathbf{q}}}, \tag{S.19}$$

where we have introduced a new symbol for the sublattice sum of the dynamical quadrupoles projected along the longitudinal direction, $\hat{\mathbf{q}}$,

$$Q^{\hat{\mathbf{q}}}_j = \sum_{\kappa\,\alpha\beta} Q^{(2,\alpha\beta)}_{\kappa j}\hat{q}_\alpha\hat{q}_\beta. \tag{S.20}$$

Note that, among the three nonanalytical terms at $O(q^2)$, only QQ survives once the double sum over the sublattices is performed; other terms (DO and dielectric dispersion) vanish because of the acoustic sum rule. By means of Martin's formula, [5]

$$e_{\alpha\beta\gamma} = \bar{e}_{\alpha\beta\gamma} + \frac{1}{\Omega}\sum_{\kappa}\Gamma^{\kappa}_{\delta\beta\gamma}Q^{(1,\alpha)}_{\kappa\delta}, \tag{S.21}$$

$$\bar{e}_{\alpha\beta\gamma} = -\frac{1}{2\Omega}\sum_{\kappa}\left(Q^{(2,\alpha\beta)}_{\kappa\gamma} + Q^{(2,\gamma\alpha)}_{\kappa\beta} - Q^{(2,\beta\gamma)}_{\kappa\alpha}\right), \tag{S.22}$$

we have the following relation to the clamped-ion piezoelectric coefficients,

$$\bar{e}^{\hat{\mathbf{q}}}_{\gamma} = \sum_{\alpha\beta}\bar{e}_{\alpha\beta\gamma}\hat{q}_\alpha\hat{q}_\beta = -\frac{1}{2\Omega}Q^{\hat{\mathbf{q}}}_{\gamma}, \tag{S.23}$$

which leads to the following result

$$\bar{K}^{\hat{\mathbf{q}}}_{jl} = \bar{K}^{\rm AN,\hat{\mathbf{q}}}_{jl} + 4\pi\Omega\frac{\bar{e}^{\hat{\mathbf{q}}}_j\,\bar{e}^{\hat{\mathbf{q}}}_l}{\hat{\mathbf{q}}\cdot\boldsymbol{\epsilon}\cdot\hat{\mathbf{q}}}. \tag{S.24}$$

This is the counterpart of Eq. (8) for "clamped-ion sound waves". To arrive at the static result, inclusive of internal strain relaxations, we need to decompose the remaining terms in Eq. (S.18) above. We have, for the piezoelectric force-response tensor,

$$\Lambda^{\kappa}_{\alpha j}(\hat{\mathbf{q}}) = \Lambda^{\mathrm{AN},\kappa}_{\alpha j}(\hat{\mathbf{q}}) - 4\pi \frac{Z^{\hat{\mathbf{q}}}_{\kappa\alpha}\, \bar{e}^{\hat{\mathbf{q}}}_{j}}{\hat{\mathbf{q}} \cdot \bar{\boldsymbol{\epsilon}} \cdot \hat{\mathbf{q}}}, \tag{S.25}$$

where the second term on the right-hand side originates from the dipole-quadrupole (DQ) interaction together with Martin's formula Eq. (S.21). Next, we have the zone-center force-constant matrix,

$$\Phi^{(0,\hat{\mathbf{q}})}_{\kappa\alpha,\kappa'\beta} = \Phi^{(0,\mathrm{AN})}_{\kappa\alpha,\kappa'\beta} + \frac{4\pi}{\Omega} \frac{Z^{\hat{\mathbf{q}}}_{\kappa\alpha}\, Z^{\hat{\mathbf{q}}}_{\kappa'\beta}}{\hat{\mathbf{q}} \cdot \bar{\boldsymbol{\epsilon}} \cdot \hat{\mathbf{q}}}. \tag{S.26}$$

Finally, by means of the Sherman-Morrison formula, [6] we can write the pseudoinverse of the latter as

$$\widetilde{\Phi}^{(0)} = \widetilde{\Phi}^{(0,\mathrm{AN})} - \frac{4\pi}{\Omega} \frac{\widetilde{\Phi}^{(0,\mathrm{AN})}|Z(\hat{\mathbf{q}})\rangle\langle Z(\hat{\mathbf{q}})|\widetilde{\Phi}^{(0,\mathrm{AN})}}{\hat{\mathbf{q}} \cdot \boldsymbol{\epsilon}_{\mathrm{static}} \cdot \hat{\mathbf{q}}}, \tag{S.27}$$

where the static dielectric tensor is given by

$$\hat{\mathbf{q}} \cdot \boldsymbol{\epsilon}_{\mathrm{static}} \cdot \hat{\mathbf{q}} = \hat{\mathbf{q}} \cdot \bar{\boldsymbol{\epsilon}} \cdot \hat{\mathbf{q}} + \frac{4\pi}{\Omega} \langle Z(\hat{\mathbf{q}})|\widetilde{\Phi}^{(0,\mathrm{AN})}|Z(\hat{\mathbf{q}})\rangle. \tag{S.28}$$

From now on we shall simplify the notation quite a bit. We need to expand the following product (we shall neglect factors of $4\pi$ and inverse volume in the following steps for clarity)

$$\begin{aligned}
\left(\langle\Lambda_j| - \frac{\bar{e}_j\langle Z|}{\bar{\epsilon}}\right)\left(\widetilde{\Phi} - \frac{\widetilde{\Phi}|Z\rangle\langle Z|\widetilde{\Phi}}{\epsilon_{\mathrm{static}}}\right)\left(|\Lambda_l\rangle - \frac{|Z\rangle\bar{e}_l}{\bar{\epsilon}}\right) = &+\langle\Lambda_j|\widetilde{\Phi}|\Lambda_l\rangle \\
&-\frac{\langle\Lambda_j|\widetilde{\Phi}|Z\rangle}{\bar{\epsilon}}\bar{e}_l - \bar{e}_j\frac{\langle Z|\widetilde{\Phi}|\Lambda_l\rangle}{\bar{\epsilon}} \\
&+\bar{e}_j\frac{\langle Z|\widetilde{\Phi}|Z\rangle}{\bar{\epsilon}^2}\bar{e}_l \\
&-\frac{\langle\Lambda_j|\widetilde{\Phi}|Z\rangle\langle Z|\widetilde{\Phi}|\Lambda_l\rangle}{\epsilon_{\mathrm{static}}} \\
&+\frac{\langle\Lambda_j|\widetilde{\Phi}|Z\rangle\langle Z|\widetilde{\Phi}|Z\rangle}{\bar{\epsilon}\epsilon_{\mathrm{static}}}\bar{e}_l \\
&+\bar{e}_j\frac{\langle Z|\widetilde{\Phi}|Z\rangle\langle Z|\widetilde{\Phi}|\Lambda_l\rangle}{\bar{\epsilon}\epsilon_{\mathrm{static}}} \\
&-\bar{e}_j\frac{\langle Z|\widetilde{\Phi}|Z\rangle\langle Z|\widetilde{\Phi}|Z\rangle}{\bar{\epsilon}^2\epsilon_{\mathrm{static}}}\bar{e}_l.
\end{aligned} \tag{S.29}$$

We can further simplify the above formula by identifying the lattice-mediated contributions to the piezoelectric and dielectric tensors, respectively,

$$\Delta e_j = \langle\Lambda_j|\widetilde{\Phi}|Z\rangle, \tag{S.30}$$

$$\Delta\epsilon = \langle Z|\widetilde{\Phi}|Z\rangle. \tag{S.31}$$

This way we have

$$\begin{aligned}
\left(\langle\Lambda_j| - \frac{\bar{e}_j\langle Z|}{\bar{\epsilon}}\right)\left(\widetilde{\Phi} - \frac{\widetilde{\Phi}|Z\rangle\langle Z|\widetilde{\Phi}}{\epsilon_{\mathrm{static}}}\right)\left(|\Lambda_l\rangle - \frac{|Z\rangle\bar{e}_l}{\bar{\epsilon}}\right) = &+\langle\Lambda_j|\widetilde{\Phi}|\Lambda_l\rangle \\
&-\frac{\Delta e_j\,\bar{e}_l + \bar{e}_j\,\Delta e_l}{\bar{\epsilon}} \\
&+\bar{e}_j\frac{\Delta\epsilon}{\bar{\epsilon}^2}\bar{e}_l \\
&-\frac{\Delta e_j \Delta e_l}{\epsilon_{\mathrm{static}}} \\
&+\frac{\Delta e_j \Delta\epsilon\bar{e}_l + \bar{e}_j\Delta\epsilon\Delta e_l}{\bar{\epsilon}\epsilon_{\mathrm{static}}} \\
&-\bar{e}_j\frac{\Delta\epsilon^2}{\bar{\epsilon}^2\epsilon_{\mathrm{static}}}\bar{e}_l.
\end{aligned} \tag{S.32}$$

The second and fifth lines, and the third and sixth can be simplified by observing that

$$1 - \frac{\Delta\epsilon}{\epsilon_{\mathrm{static}}} = \frac{\bar{\epsilon}}{\epsilon_{\mathrm{static}}}, \tag{S.33}$$

which leads to the following

$$\left(\langle\Lambda_j| - \frac{\bar{e}_j\langle Z|}{\bar{\epsilon}}\right)\left(\widetilde{\Phi} - \frac{\widetilde{\Phi}|Z\rangle\langle Z|\widetilde{\Phi}}{\epsilon_{\text{static}}}\right)\left(|\Lambda_l\rangle - \frac{|Z\rangle\bar{e}_l}{\bar{\epsilon}}\right) = +\langle\Lambda_j|\widetilde{\Phi}|\Lambda_l\rangle - \frac{\Delta e_j\,\bar{e}_l + \bar{e}_j\,\Delta e_l}{\epsilon_{\text{static}}} + \bar{e}_j\frac{\Delta\epsilon}{\bar{\epsilon}\epsilon_{\text{static}}}\bar{e}_l - \frac{\Delta e_j\Delta e_l}{\epsilon_{\text{static}}}. \tag{S.34}$$

We shall combine the last three terms together with the nonanalytic part of the second-order term, eventually obtaining

$$\frac{\bar{e}_j\bar{e}_l}{\bar{\epsilon}} - \bar{e}_j\frac{\Delta\epsilon}{\bar{\epsilon}\epsilon_{\text{static}}}\bar{e}_l + \frac{\Delta e_j\Delta e_l}{\epsilon_{\text{static}}} + \frac{\Delta e_j\,\bar{e}_l + \bar{e}_j\,\Delta e_l}{\epsilon_{\text{static}}} = \frac{e_j\,e_l}{\epsilon_{\text{static}}}. \tag{S.35}$$

By putting all pieces together, we find

$$K_{jl}^{\hat{\mathbf{q}}} = K_{jl}^{\text{AN},\hat{\mathbf{q}}} + 4\pi\Omega\frac{e_j^{\hat{\mathbf{q}}}\,e_l^{\hat{\mathbf{q}}}}{\hat{\mathbf{q}}\cdot\boldsymbol{\epsilon}\cdot\hat{\mathbf{q}}}, \tag{S.36}$$

where

$$K_{jl}^{\text{AN},\hat{\mathbf{q}}} = \bar{K}_{jl}^{\text{AN},\hat{\mathbf{q}}} - \sum_{\kappa\kappa'\alpha\beta}\Lambda_{\kappa\alpha j}^{\text{AN}}(\hat{\mathbf{q}})\,\widetilde{\Phi}_{\kappa\alpha,\kappa'\beta}^{(0,\text{AN})}\,\Lambda_{\kappa'\beta l}^{\text{AN}}(\hat{\mathbf{q}}). = \Omega\sum_{ik}C_{ijkl}\hat{q}_i\hat{q}_k, \tag{S.37}$$

thus recovering the macroscopic Christoffel equation in electromechanically active crystals, Eq. (4) of the main text. This result demonstrates that the explicit treatment of DQ and QQ interactions is essential in piezoelectric crystals for correctly describing the contribution of macroscopic electric fields to the sound velocity.

**Computational parameters.** DFT and DFPT calculations have been carried out using ABINIT [7, 8] within the Perdew-Wang parametrizaion of the local density approximation (LDA). [9] Norm-conserving pseudopotentials of the Troullier-Martins type have been employed for all atom types. Six, ten and twelve valence electrons have been considered explicitly in O, Ba and Ti, respectively.

The rhombohedral crystal structure of $BaTiO_3$ has been simulated employing a primitive unit cell of five atoms sampled with Monkhorst-Pack mesh of $8 \times 8 \times 8$ or $12 \times 12 \times 12$ **k**-points and a plane-wave cut-off of 100 Ha. With these settings, the unit cell has been relaxed until forces were smaller than $5{\cdot}10^{-5}$ Ha/Bohr and the optimized lattice parameter $a$ and the angle $\alpha$ of the rhombohedral cell have been found to be 3.944 Å and 89.91°, respectively.

Dynamical quadrupoles are calculated based on a recent DFPT scheme developed by two of us. [3, 10] Octupoles and dielectric dispersion tensor have been calculated by performing a numerical fit of the charge response to a phonon or scalar potential, respectively, on a mesh of **q** points surrounding Γ. The macroscopic component of the electrostatic screening was switched off during the self-consistent cycles, following the prescriptions of Refs.1 and 11. All relevant tensor components are provided in atomic units and along Cartesian directions the Tables below. [The primitive translation vectors of the $R3m$ cell were chosen as $\mathbf{a}_1 = (r, s, s)$; $\mathbf{a}_2 = (s, r, s)$; $\mathbf{a}_3 = (s, s, r)$.] The dynamic quadrupoles have been validated by benchmarking the clamped-ion piezoelectric tensor obtained from their atomic sublattice summation (via Eq. (S.22)) against the corresponding value obtained from a strain and electric field response DFPT calculation [12] (see Table S.III). The dynamic octupoles, in turn, have been validated by comparing the clamped-ion flexoelectric coefficients that can be calculated from the sublattice summation of the octupolar moments following the prescriptions of Refs 13 and 14 with the corresponding values obtained by a long-wave DFPT calculation [3, 10] (see Table S.IV).

TABLE S.I. Cartesian components of the **clamped-ion dielectric tensor**, $\epsilon_{\alpha\beta}$ and the **dielectric dispersion tensor**, $\epsilon^{(4)}_{\alpha\beta,\gamma\delta}$. Atomic units are used; only linearly independent coefficients are shown.

| $\epsilon_{xx}$ | $\epsilon_{xy}$ | $\epsilon^{(4)}_{xxxx}$ | $\epsilon^{(4)}_{xxyy}$ | $\epsilon^{(4)}_{xxxy}$ | $\epsilon^{(4)}_{xxyz}$ |
|---|---|---|---|---|---|
| 6.083 | -0.111 | −30.159 | −7.104 | 0.561 | 0.088 |

TABLE S.II. Cartesian components of **dynamical multipole tensors**. Atomic untis are used; only linearly independent coefficients are shown.

| | $\kappa$ = Ba | $\kappa$ = Ti | $\kappa$ =$O_0$ | $\kappa$ =$O_2$ | $\kappa$ =$O_3$ |
|---|---|---|---|---|---|
| $Q^{(1,x)}_{\kappa x}$ | 2.786 | 6.500 | −5.200 | −2.043 | −2.043 |
| $Q^{(1,y)}_{\kappa x}$ | −0.011 | −0.226 | 0.168 | 0.074 | −0.006 |
| $Q^{(1,z)}_{\kappa x}$ | −0.011 | −0.226 | 0.168 | −0.006 | 0.074 |
| $Q^{(2,xx)}_{\kappa x}$ | −1.060 | 1.560 | −2.175 | −0.843 | −0.843 |
| $Q^{(2,xy)}_{\kappa x}$ | 0.468 | −0.317 | 1.420 | −0.120 | 0.020 |
| $Q^{(2,xz)}_{\kappa x}$ | 0.468 | −0.317 | 1.420 | 0.020 | −0.120 |
| $Q^{(2,yy)}_{\kappa x}$ | −0.102 | 1.566 | −1.561 | 1.167 | −0.069 |
| $Q^{(2,yz)}_{\kappa x}$ | 0.004 | −0.059 | 0.010 | −0.044 | −0.044 |
| $Q^{(2,zz)}_{\kappa x}$ | −0.102 | 1.566 | −1.561 | −0.069 | 1.167 |
| $Q^{(3,xxx)}_{\kappa x}$ | −285.161 | 94.437 | −328.941 | −106.134 | −106.134 |
| $Q^{(3,xxy)}_{\kappa x}$ | 3.699 | −2.380 | 5.982 | 2.294 | 0.849 |
| $Q^{(3,xxz)}_{\kappa x}$ | 3.699 | −2.380 | 5.982 | 0.849 | 2.294 |
| $Q^{(3,xyy)}_{\kappa x}$ | −84.574 | −38.987 | −70.265 | −38.317 | −35.231 |
| $Q^{(3,xyz)}_{\kappa x}$ | 1.273 | 1.720 | 0.642 | 0.165 | 0.165 |
| $Q^{(3,xzz)}_{\kappa x}$ | −84.574 | −38.987 | −70.265 | −35.231 | −38.317 |
| $Q^{(3,yyy)}_{\kappa x}$ | −0.650 | −8.638 | 8.095 | 4.220 | −0.106 |
| $Q^{(3,yyz)}_{\kappa x}$ | 0.006 | −0.848 | 0.755 | 0.004 | 0.718 |
| $Q^{(3,yzz)}_{\kappa x}$ | 0.006 | −0.848 | 0.755 | 0.718 | 0.004 |
| $Q^{(3,zzz)}_{\kappa x}$ | −0.650 | −8.638 | 8.095 | −0.106 | 4.220 |

TABLE S.III. Linearly independent **clamped-ion piezoelectric coefficients** (in $mC/m^2$) calculated via two different methods. "Quadrupoles": from the lattice summation of quadrupole moments via Eq. (S.22), "Strain": standard DFPT approach relying on the strain and electric field response. [12]

| | $\bar{e}_{xxx}$ | $\bar{e}_{xyy}$ | $\bar{e}_{xxy}$ | $\bar{e}_{xyz}$ |
|---|---|---|---|---|
| Quadrupoles | 232.3251 | −134.0335 | −69.2064 | 9.1963 |
| Strain | 232.3253 | −134.0372 | −69.2050 | 9.1963 |

TABLE S.IV. **Multipolar sum rule for the clamped-ion flexoelectric tensor.** The lattice summation of dynamic octupole moments is compared with the flexoelectric tensor components obtained via a long-wave DFPT approach. [3] "Octupoles" shows $O^{\text{oct}}_{\beta,\alpha\gamma\delta} = \sum_\kappa Q^{(3,\alpha\gamma\delta)}_{\kappa\beta}/2\Omega$ [13, 15, 16]. "LW DFPT" shows the same physical quantity calculated as $O^{\text{LW}}_{\beta,\alpha\gamma\delta} = \bar{\mu}^{\text{I}}_{\alpha\beta,\gamma\delta} + \bar{\mu}^{\text{I}}_{\gamma\beta,\delta\alpha} + \bar{\mu}^{\text{I}}_{\delta\beta,\alpha\gamma}$, with $\bar{\mu}^{\text{I}}_{\alpha\beta,\gamma\delta}$ being the type-I clamped-ion flexoelectric coefficients obtained from the analytical momentum derivative of the second-order strain and electric field response. [3] Units are nC/m; only linearly independent coefficients are shown.

| | $x, xxx$ | $x, xxy$ | $x, xyy$ | $x, yyy$ | $x, xyz$ | $x, yyz$ |
|---|---|---|---|---|---|---|
| Octupoles | −2.677 | 0.038 | −0.978 | 0.011 | 0.014 | 0.002 |
| LW DFPT | −2.689 | 0.038 | −0.982 | 0.011 | 0.015 | 0.002 |

TABLE S.V. **$BaTiO_3$ velocity of sound** (in km/s) in the directions [100], [110] and [111] calculated from macroscopic elasticity arguments (Eqs (4), (7) and (8) of the manuscript). The last three columns show the estimated velocities when macroscopics electric fields are neglected, i.e., just the first term at the rhs of Eq. 8 is included in the elastic tensor.

| | With el. fields | | | Without el. fields | | |
|---|---|---|---|---|---|---|
| | $v_{s,1}$ | $v_{s,2}$ | $v_{s,3}$ | $v_{s,1}$ | $v_{s,2}$ | $v_{s,3}$ |
| [100] | 4.504 | 4.528 | 6.937 | 4.422 | 4.528 | 5.349 |
| [110] | 2.000 | 4.489 | 7.308 | 2.000 | 4.481 | 6.428 |
| [111] | 2.852 | 2.852 | 7.411 | 2.852 | 2.852 | 6.773 |

TABLE S.VI. Clamped-ion, lattice-mediated and total **$BaTiO_3$ and GaP piezoelectric tensors** calculated via DFPT approach relying on the strain and electric field response. [12] Units are $C/m^2$; only linearly independent coefficients are shown.

| | $BaTiO_3$ | | | | GaP |
|---|---|---|---|---|---|
| | $e_{xxx}$ | $e_{xyy}$ | $e_{xyz}$ | $e_{xxy}$ | $e_{xyz}$ |
| CI | 0.232 | -0.134 | 0.009 | -0.069 | -0.762 |
| LM | -9.270 | 1.393 | 0.281 | -0.498 | 0.669 |
| TOT | -9.037 | 1.259 | 0.290 | -0.568 | -0.093 |

FIG. S.1. **$BaTiO_3$ velocity of sound** of the three acoustic branches along the [100] (a-c) and [111] (d-f) directions as a function of the **q**-point mesh. Dotted horizontal lines indicate the reference value of the sound velocity, obtained from macroscopic elasticity. Different symbols (lines are a guide to the eye) show the velocities as obtained by considering an increasing number of multipolar interactions in the long-range dynamical matrix.

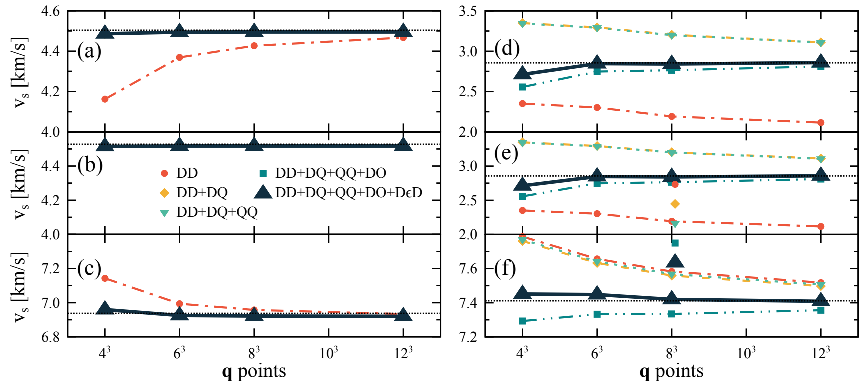


FIG. S.2. **GaP velocity of sound** of the three acoustic branches as a function of the **q**-point mesh. Velocities along the [100] (a-c), the [110] (d-f) and the [111] (g-i) directions are shown. Doted-horizontal lines indicate the value of the sound velocity obtained from macroscopic elasticity. Different symbols (lines are a guide to the eye) in each panel show the velocities as obtained by considering an increasing number of multipolar interactions in the long-range dynamical matrix.

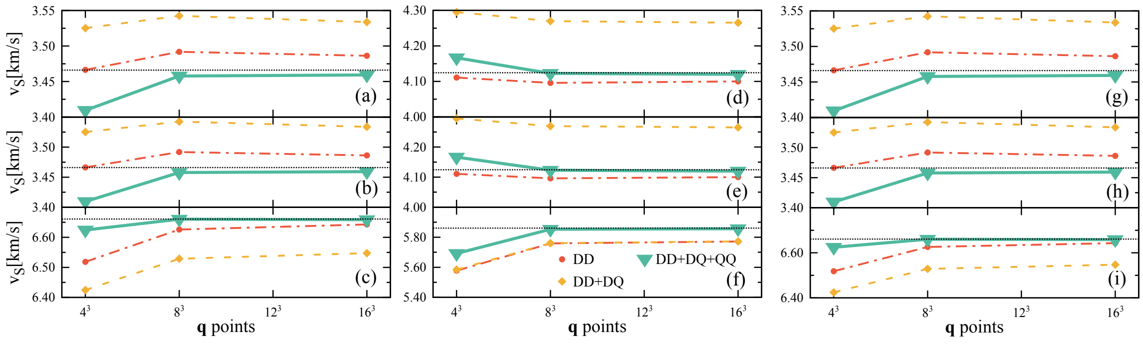

[1] M. Stengel, Physical Review B **88**, 174106 (2013).
[2] M. Stengel, Physical Review B **93**, 245107 (2016).
[3] M. Royo and M. Stengel, Phys. Rev. X **9**, 021050 (2019).
[4] X. Gonze and C. Lee, Physical Review B **55**, 10355 (1997).
[5] R. M. Martin, Physical Review B **5**, 1607 (1972).
[6] W. H. Press, S. a. Teukolsky, W. T. Vetterling, and B. P. Flannery, *Numerical Recipes in Fortran 77: the Art of Scientific Computing. Second Edition*, Vol. 1 (1996) Chap. 2, p. 65.
[7] X. Gonze, B. Amadon, P.-M. Anglade, J.-M. Beuken, F. Bottin, P. Boulanger, F. Bruneval, D. Caliste, R. Caracas, M. Côté, T. Deutsch, L. Genovese, P. Ghosez, M. Giantomassi, S. Goedecker, D. Hamann, P. Hermet, F. Jollet, G. Jomard, S. Leroux, M. Mancini, S. Mazevet, M. Oliveira, G. Onida, Y. Pouillon, T. Rangel, G.-M. Rignanese, D. Sangalli, R. Shaltaf, M. Torrent, M. Verstraete, G. Zerah, and J. Zwanziger, Computer Physics Communications **180**, 2582 (2009).
[8] X. Gonze, F. Jollet, F. A. Araujo, D. Adams, B. Amadon, T. Applencourt, C. Audouze, J.-M. Beuken, J. Bieder, A. Bokhanchuk, E. Bousquet, F. Bruneval, D. Caliste, M. Côté, F. Dahm, F. D. Pieve, M. Delaveau, M. D. Gennaro, B. Dorado, C. Espejo, G. Geneste, L. Genovese, A. Gerossier, M. Giantomassi, Y. Gillet, D. Hamann, L. He, G. Jomard, J. L. Janssen, S. L. Roux, A. Levitt, A. Lherbier, F. Liu, I. Lukačević, A. Martin, C. Martins, M. Oliveira, S. Poncé, Y. Pouillon, T. Rangel, G.-M. Rignanese, A. Romero, B. Rousseau, O. Rubel, A. Shukri, M. Stankovski, M. Torrent, M. V. Setten, B. V. Troeye, M. Verstraete, D. Waroquiers, J. Wiktor, B. Xu, A. Zhou, and J. Zwanziger, Computer Physics Communications **205**, 106 (2016).
[9] J. P. Perdew and Y. Wang, Physical Review B **45**, 13244 (1992).
[10] A. H. Romero, D. C. Allan, B. Amadon, G. Antonius, T. Applencourt, L. Baguet, J. Bieder, F. Bottin, J. Bouchet, E. Bousquet, F. Bruneval, G. Brunin, D. Caliste, M. Côté, J. Denier, C. Dreyer, P. Ghosez, M. Giantomassi, Y. Gillet, O. Gingras, D. R. Hamann, G. Hautier, F. Jollet, G. Jomard, A. Martin, H. P. C. Miranda, F. Naccarato, G. Petretto, N. A. Pike, V. Planes, S. Prokhorenko, T. Rangel, F. Ricci, G.-M. Rignanese, M. Royo, M. Stengel, M. Torrent, M. J. van Setten, B. Van Troeye, M. J. Verstraete, J. Wiktor, J. W. Zwanziger, and X. Gonze, The Journal of Chemical Physics **152**, 124102 (2020).
[11] X. Wu, D. Vanderbilt, and D. R. Hamann, Phys. Rev. B **72**, 035105 (2005).
[12] D. R. Hamann, X. Wu, K. M. Rabe, and D. Vanderbilt, Physical Review B **71**, 035117 (2005).
[13] R. Resta, Phys. Rev. Lett. **105**, 127601 (2010).
[14] J. Hong and D. Vanderbilt, Phys. Rev. B **84**, 180101(R) (2011).
[15] J. Hong and D. Vanderbilt, Phys. Rev. B **88**, 174107 (2013).
[16] M. Stengel and D. Vanderbilt, in *Flexoelectricity in Solids From Theory to Applications*, edited by A. K. Tagantsev and P. V. Yudin (World Scientific Publishing Co., Singapore, 2016) Chap. 2, pp. 31–110.
